# Supplementary material for: Apply Non-Hermitian Physics to Realize Ultra-High-Quality Factors of Optically Trapped Particles
Source: arXiv:2308.16502 source file (2023-08-31)
Supplement: Supplementary file 1 [file SupplementaryMaterials.pdf]

## Supplementary Materials

After substituting the particular solution for the $i$-th mode $q_i = q_{i0}e^{-i\omega_i t}$ into Eq. (4) of the main text, we obtain the following equation:

$$m\omega_i^2 + K_i + i\gamma\omega_i = 0, \tag{s1}$$

where $K_i$ represents the $i$-th eigenvalue of the force constant matrix, and $\gamma$ is the damping coefficient of the ambient medium.

From Eq. , one could solve the particle vibration frequency $\omega_i$:

$$\begin{cases} \omega_{i,+} = \frac{-i\gamma}{2m} + \sqrt{\frac{-K_i}{m} - \left(\frac{\gamma}{2m}\right)^2} \\ \omega_{i,-} = \frac{-i\gamma}{2m} - \sqrt{\frac{-K_i}{m} - \left(\frac{\gamma}{2m}\right)^2} \end{cases}. \tag{s2}$$

For the sake of simplicity, we express the second terms on the right-hand side of Eq. as $\sqrt{\frac{-K_i}{m} - \left(\frac{\gamma}{2m}\right)^2} = \omega_i' + i\omega_i''$, where $\omega_i'$ and $\omega_i''$ represent the real and imaginary parts, respectively. It is evident that the vibration frequencies $\omega_{i,+}$ and $\omega_{i,-}$ exhibit distinct imaginary components: $\mathrm{Im}[\omega_{i,+}] = \frac{-i\gamma}{2m} + i\omega_i''$ and $\mathrm{Im}[\omega_{i,-}] = \frac{-i\gamma}{2m} - i\omega_i''$. The imaginary parts of the vibration frequencies are governed by the competition between the values of $\frac{-K_i}{m}$ and $\left(\frac{\gamma}{2m}\right)^2$, whereas their real parts are of opposite signs while sharing the same absolute value for each $i$: $|\mathrm{Re}[\omega_{i,+}]| = |\mathrm{Re}[\omega_{i,-}]| = |\omega'|$.

In this study, we employ optical trapping as a case study (to refer Fig. 1(**a**) and Fig. 1(**b**) in the main text), specifically focusing on a single silica particle with a radius of 0.5 μm and refractive index of 1.45. The particle is trapped by two counter-propagating Gaussian beams within a low vacuum environment with a pressure of 10 Torr. The polarization state of the beams is defined as $\hat{\boldsymbol{p}} = \hat{\boldsymbol{x}}cos\xi + i\hat{\boldsymbol{y}}sin\xi$, where ξ=0 ° corresponds to linear polarization (Fig. 1(**a**)), and ξ=45° represents circular polarization (Fig. 1(**b**)). Notably, the motion of the particle in the transverse direction is decoupled from the $z$-direction. Focusing solely on the transverse motion, we analyze the force constant matrix $\overleftrightarrow{\mathbf{K}}_{2D}$, which yields two

eigenvalues, $K_{i=1,2}$, and consequently results in four vibration frequencies, namely, $\omega_{1,+}$, $\omega_{1,-}$, $\omega_{2,+}$ and $\omega_{2,-}$, as depicted in Fig. S1. As the beam polarization angle varies from linear (ξ=0°) to circular (ξ=45°), an exceptional point (EP) is observed at ξ≈18°. Referring to the definition of the Q factor of the *i*-th mode $\mathrm{Q}_i =-\frac{|\mathrm{Re}[\omega_i]|}{2\mathrm{Im}[\omega_i]}$, we consider the Q factors corresponding to $\omega_{i,+}$ and $\omega_{i,-}$ by classification of eigenvalues $K_i$ as following:

(i) Prior to the EP occurrence, the eigenvalues $K_i$ correspond to two distinct real values (*i*=1,2). Under the conditions of a low vacuum with a pressure of 10 Torr, the inequality $\frac{-K_i}{m} \geq \left(\frac{\gamma}{2m}\right)^2$ holds true, which implies that $\sqrt{\frac{-K_i}{m} - \left(\frac{\gamma}{2m}\right)^2} = \omega'$. Consequently, the vibration frequencies exhibit identical imaginary parts ($\mathrm{Im}[\omega_{i,+}] = \mathrm{Im}[\omega_{i,-}] = \frac{-i\gamma}{2m}$) as well as equal absolute real parts of vibration frequencies ($\mathrm{Re}[\omega_{i,+}] = \mathrm{Re}[\omega_{i,-}]$), as illustrated in Fig. S1 (before EP). Thus, it follows that the *i*-th mode with real $K_i$ generates the same Q factor ($\mathrm{Q}_{i,+} = \mathrm{Q}_{i,-}$) in a low vacuum setting.

(ii) After the EP occurrence, the eigenvalues $K_i$ form a complex conjugate pair. Irrespective of the damping coefficient, the second terms on the right-hand side of Eq. remain $\sqrt{\frac{-K_i}{m} - \left(\frac{\gamma}{2m}\right)^2} = \omega_i' + i\omega_i''$. The vibration frequencies are denoted as $\omega_{i,+} = \omega_i' + i(\omega_i'' - \frac{\gamma}{2m})$ and $\omega_{i,-} = -\omega_i' - i(\omega_i'' - \frac{\gamma}{2m})$. Importantly, it is observed that for the modes with $K_1 = K_2^*$, the absolute values of the real parts of the vibration frequencies are the same, i.e., $|\mathrm{Re}[\omega_{1,+}]| = |\mathrm{Re}[\omega_{1,-}]| = |\mathrm{Re}[\omega_{2,+}]| = |\mathrm{Re}[\omega_{2,-}]|$, whereas $\mathrm{Im}[\omega_{1,+}] = \mathrm{Im}[\omega_{2,-}]$ and $\mathrm{Im}[\omega_{1,-}] = \mathrm{Im}[\omega_{2,+}]$, as depicted in Fig. S1 (after EP). Consequently, we can derive that $\mathrm{Q}_{1,+} = \mathrm{Q}_{2,-}$ and $\mathrm{Q}_{1,-} = \mathrm{Q}_{2,+}$.

In conclusion, in the context of a low vacuum environment, we may opt for a simplified approach by concentrating exclusively on the vibration frequency $\omega_{i,+}$ rather than considering both $\omega_i = \omega_{i,+}$ and $\omega_i = \omega_{i,-}$. Throughout this manuscript,

we adopt the notation $\omega_i = \omega_{i,+}$ due to the comprehensive representation of the Q factor, encompassing both $Q_{i,+}$ and $Q_{i,-}$.

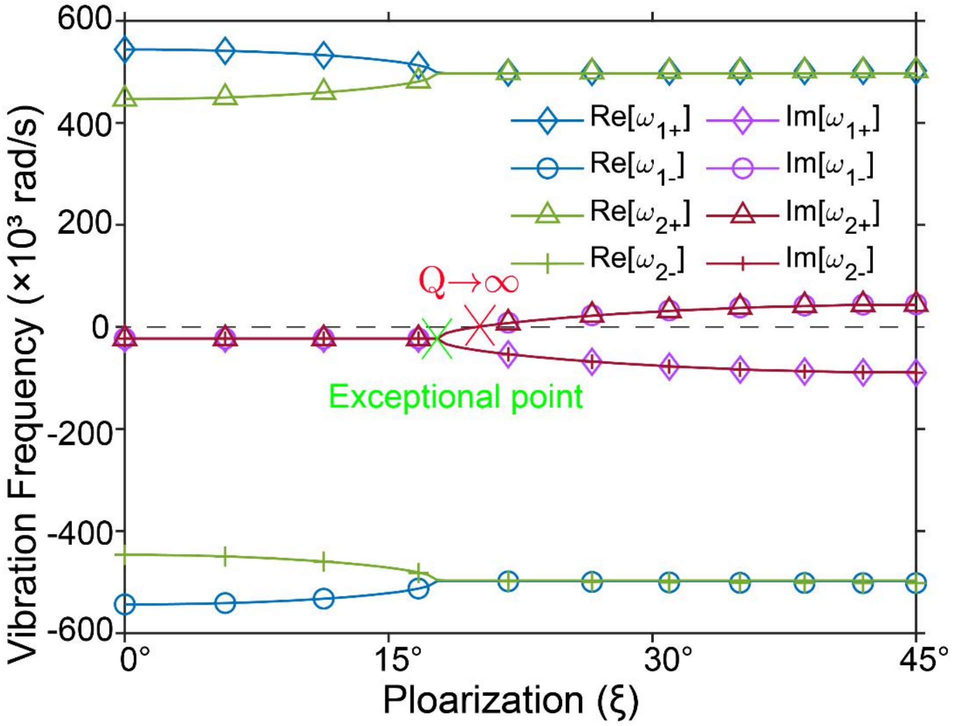


Figure S1. Vibration frequencies of optically trapped silica particles in a low vacuum environment. The figure illustrates the investigation of optically trapped silica particles (with a radius of $r$ = 0.5 μm and a refractive index $n$ = 1.45) in a low vacuum with an ambient pressure of 10 Torr. The polarization ($\hat{\boldsymbol{p}} = \hat{\boldsymbol{x}} cos\xi + i\hat{\boldsymbol{y}} sin\xi$) of the counter-propagating incident Gaussian beams is systematically varied, ranging from linear (ξ = 0°) to circular (ξ = 45°) polarization. The incident beams, characterized by a wavelength of $\lambda = 1.064$ μm, are focused by an objective lens with a numerical aperture (NA) of 0.9, each having a normalized power of 1 mW. The figure displays the real ($\mathrm{Re}[\omega_{1,+}]$ and $\mathrm{Re}[\omega_{1,-}]$) and the imaginary ($\mathrm{Im}[\omega_{1,+}]$ and $\mathrm{Im}[\omega_{1,-}]$) parts of the vibration frequency corresponding to the *1st* mode, represented by the blue and purple lines, respectively. Additionally, the green and red lines depict the real ($\mathrm{Re}[\omega_{2,+}]$ and $\mathrm{Re}[\omega_{2,-}]$) and the imaginary ($\mathrm{Im}[\omega_{2,+}]$ and $\mathrm{Im}[\omega_{2,-}]$) parts of the vibration frequency corresponding to the *2nd* mode.
